# Supplementary material for: MLPerf Power: Benchmarking the Energy Efficiency of Machine Learning Systems from Microwatts to Megawatts for Sustainable AI
Source: arXiv:2410.12032 source file (2025-02-06)
Supplement: Supplementary file 1 [file appendix.tex]

\section{Artifact Appendix}

\subsection{Abstract}

Here, we include the steps and resources to reproduce each contribution of the MLPerf Power paper. Refer to our Github repository\footnote{\label{repo}\url{https://github.com/aryatschand/MLPerf-Power-HPCA-2025}} for more details. 

Based on our outlined contributions in the Introduction section of out paper, we provide the following resources in this appendix:
\begin{itemize}
    \item To collect power measurements using the proposed methodology, refer to the \textit{measurement\_tutorial}\footnote{\label{measurement}\url{https://github.com/aryatschand/MLPerf-Power-HPCA-2025/blob/main/measurement_tutorial.md}} markdown file. This will provide you a tutorial with the exact steps to measure the power of any system using the MLPerf Power methodology. 
    
    \item Collecting power measurements require a significant setup cost. Due to this limitation, we understand that it may be infeasible to reproduce the power measurement methodology in the scope of the artifact evaluation. We provide our MLPerf Power dataset of over 1,800 submissions from companies that implement this methodology to measure their own systems for evaluation of this artifact.
    
    \item We include the source code to reproduce all results, figures, and insights in the MLPerf Power paper.
\end{itemize}

The sections of the artifact appendix that follow assume the usage of our publicly accessibly MLPerf Power data that has already been pre-collected using the methodology that we provide in the artifact.

If you want to measure it yourself, we provide the resources to do so.

In case you want to measure your own system and add your own power measurements to the evaluation, we provide the supplemental resources\footnote{\url{https://github.com/mlcommons/power-dev}} to do so, although this is not explicitly part of our artifact.

\subsection{Artifact check-list}
\begin{itemize}
    \item \textbf{Program: }Data processing and figure generation code for Figures 1, 2, 5a-c, 6, 7, 8, 9, 10, and 11a-b in the paper and their corresponding insights.
    \item \textbf{Data set: }Raw and filtered MLPerf Power data.
    \item \textbf{Run-time environment: }Docker version 27.3.1.
    \item \textbf{Output: }All figures in the paper reproduced in a local directory.
    \item \textbf{Publicly available: }Yes
\end{itemize}

\subsection{Access}
All of our source code for MLPerf Power can be obtained via our Github repository\footref{repo} with the data and figure reproduction here.

\subsection{Dependencies}
Docker version 27.3.1 must be installed on a machine running MacOS or Linux to execute the figure reproduction container. There are no other hardware dependencies to reproduce the work. Refer to the Appendix Extensions section for power analyzer hardware dependencies for power measurement.

\subsection{Workflow and Results}
\textbf{Data: } These steps of our power measurement methodology were followed by every public MLPerf power submission and were meticulously verified in a 2-step auditing process by MLPerf.

All data (except for Figure 11b) is publicly accessible on the MLCommons benchmarks website under \textit{Closed - Power}. Now, you can access every submission with submitted power measurements across every MLPerf version and division benchmark.

The raw data dumped from the MLPerf benchmark website can be found in \textit{raw\_data.csv}. This contains all power and performance data from all submission divisions. This raw data is an aggregation from exporting all data directly from the website. Between the public data found on the website and the raw data file, there is no data processing beyond a simple aggregation.

This data is cleaned, filtered by division, and dumped into \textit{/code/data\_cleaned\_\{division.csv\}}. This process only involves filtering our rows that do not fit the division or do not contain power measurements, and filtering our columns that contain data that is not relevant for system identification and evaluation. This data is used to create the figures in the paper, and all pre-processing work to calculate the data displayed in the graph can be found in the figure's corresponding python file in the \textit{/code} directory.

For a more detailed description of each figure in the paper and the specific MLPerf power data points used for each, refer to the \textit{figures} \footnote{\url{https://github.com/aryatschand/MLPerf-Power-HPCA-2025/blob/main/figures.md}} markdown file.

\textbf{Installation: } Once Docker is installed, simply follow the instructions in our repository README \footnote{\label{readme}\url{https://github.com/aryatschand/MLPerf-Power-HPCA-2025/blob/main/README.md}}. The 

\begin{verbatim}
    ./run\_docker
\end{verbatim}

\noindent
 script will build a docker container with the cleaned MLPerf Power data, figure code, and all required dependencies. It will then run all the code to create each figure in the container, create a new 'figures' directory locally on your machine, and copy all the figures over. Once the script is done executing. You can inspect the post-processed data and generated figures and verify that they match the paper.

Optionally, you can also run the code for each figure individually. Refer to the README\footref{readme} for information on how to do this.

\subsection{Extensions}

\textbf{Power measurement dependencies: }
If you are interested in implementing the proposed power measurement methodology, the SPEC PTDaemon tool and a SPEC PTDaemon-certified power analyzer is required. Yokogawa is the one that most submitters have submitted with and a new single-channel model like 310E can cost around 3000\$. The MLCommons taskforce on automation and reproducibility is also using the Yokogawa 310E alongside the Collective Mind framework to automate and simplify MLPerf submissions~\cite{cm4mlperf}. 

Because of the significant dependencies to implement this methodology, we do not include this in our artifact but provide all instructions, code, and online resources necessary to measure the power consumption of any system.

If you are interested in exploring our power measurement methodology tutorial, you can refer to the \textit{measurement\_tutorial} \footref{measurement} markdown file. In that file, we also provide an specific example power measurement from MLPerf Training v4.0.

\textbf{Future usage: }
We encourage users to build on our analysis and draw deeper insights from the MLPerf Power submission data. We anticipate that there is still much to learn about energy efficiency optimizations from the data and logs.

\subsection{Methodology}
Submission, reviewing and badging methodology:
\begin{itemize}
    \item \url{http://ctuning.org/ae/submission-20190109.html}
    \item \url{http://ctuning.org/ae/reviewing-20190109.html}
    \item \url{https://www.acm.org/publications/policies/artifact-review-badging}
\end{itemize}
